# Supplementary material for: Bifurcation Identification for Ultrasound-driven Robotic Cannulation
Source: arXiv:2409.06817 source file (2024-09-10)
Supplement: Supplementary file 1 [file Appendix.tex]

%  % Algorithm: Erode
% \begin{algorithm}
% \caption{Erosion of Segmentation Mask}
% \label{alg:erosion}
% \begin{algorithmic}[1]
%     \Require $\text{$M_{s}$}$: binary segmentation mask %containing $\in \{0, 1\}$
%     \Require $\text{$n$}$ = 3 \#kernel size
%     \Require $\text{$\delta_{s}$}$: vessel radius threshold used as stopping criteria
%     %\Require $\text{$\delta_{n}$}$: vessel radius threshold used to filter out noise
%     \State \text{initialize kernel $K$ of size $n \times n$ with $1$'s}
%     %\If{\text{not} \Call{detect\_circles}{$\text{$LabelMask$}$}}
%     %    \State \textbf{return} $\text{$LabelMask$}$
%     %\EndIf
%     \While{\Call{minEnclosingCircle\footnotemark}{$M_{s}$} $>$ $\delta_{s}$}
%         \State $\text{$M_{s}$} \gets$ {$\text{$M_{s} * K$}$} \Comment{$\text{$M_{s}$}$ dimensions preserved}
%         \State $\text{$M_{s}$} \gets$ standardize $\text{$M_{s}$}$ \Comment{$\text{$M_{s}$} \in [0, 1]$}
%         \State $\text{$M_{s}$} \gets$ binarize $\text{$M_{s}$}$ \Comment{$\text{$M_{s}$} \in \{0, 1\}$}
%     \EndWhile
%     \State \textbf{return} $\text{$M_{s}$}$
%     \end{algorithmic}
% \end{algorithm}

% \begin{table}
% \vspace{-2pt}
% \caption{Comparing BIFURC with other methods}
% \begin{tabularx}{\columnwidth}{l*{5}{X}}
% \toprule
%  & \textbf{Fully Autonomous} & \textbf{Vessel} & \textbf{Modality} & \textbf{Test Subjects} & \textbf{Reported Performance}\\
% \midrule
% Chen\cite{Chen2020Feb} & \checkmark & Peripheral & VIR, US & Rat, Arm Vessel & 88.2\% \\
% \midrule
% CathBot\cite{Cheng2019Jan} & \textbf{x} & Peripheral & Electrical Impedance & Phantom & 86\% \\
% \midrule
% Leipheimer\cite{leipheimer2019first} & \textbf{x} & Peripheral & US, NIR & 31 Humans & 87\% \\
% \midrule
% AI Guide\cite{bios11120522} & \textbf{x} & Femoral & US & Phantom, 3 Pigs (Hypotensive) & 78\% \\
% \midrule
% Experts\cite{Seto} & \textbf{x} & Femoral & US & 1,004 Humans & 83\% \\
% \midrule
% BIFURC & \checkmark & Femoral & US & Phantom, 6 Pigs (Unhealthy) & 85.7\% \\
% \bottomrule
% \end{tabularx}
% \label{tab:comparison-with-bifurc}
% \vspace{-2pt}
% \end{table}



% % Algorithm: Erode
% \begin{algorithm}[H]
% \vspace{-2pt}
% \caption{Merging Segments}
% \label{alg:merging}
% \begin{algorithmic}[1]
%     \Require $\text{segments}$: List of segments.
%     % \Require $\text{$\delta_{d}$}$: Distance threshold for interpolation.
%     \Require $\text{$\delta_{h}$}$: Difference in height threshold (planar check).
%     \Require $\text{$\delta_{\theta}$}$: Difference in angle threshold (planar check).
%     \Require $\text{$\epsilon_{i}$}$: Floating point tolerance (parallel line check).
%     \Require $\text{$\delta_{sd}$}$: Minimum distance between best-fit lines.
%     \State \text{mergeablePairs} $\gets$ \text{Initialize empty list.}
%     % \For{\text{each segment in segments}}
%     %     \State \Call{\text{interpolate}}{\text{segment}, $\delta_{d}$}
%     % \EndFor
%     \State \text{segmentPairs} $\gets$ \Call{\text{getUniquePairs}}{\text{segments}}
%     \State $n$ $\gets$ \Call{\text{length}}{\text{segmentPairs}}
%     \For{$i \gets 1$ to $n$}
%         \State \text{pair} $\gets$ \text{segmentPairs[i]}
%         \If{\Call{\text{isSamePlane}}{\text{pair}, $\delta_{h}$, $\delta_{\theta}$}}
%             \State \text{intersection} $\gets$ \Call{\text{findIntersection}}{\text{pair}, $\epsilon_{i}$}
%             \State \text{bounded} $\gets$ \Call{\text{isBounded}}{\text{pair}, \text{segments}}
%             \If{\text{intersection exists} $\land$ \text{bounded}}
%                 \If{\Call{\text{isClose}}{\text{pair}, $\delta_{sd}$}}
%                     \State \text{mergeablePairs} $\gets$ \text{mergeablePairs} $+$ \text{pair}
%                 \EndIf
%             \EndIf
%         \EndIf
%     \EndFor
%     \State \text{cComponents} $\gets$ \Call{\text{getComponents}}{\text{mergeablePairs}} \Comment{Find connected components}
%     \State \text{segmentAdjMatrix} $\gets$ \Call{\text{buildGraph}}{\text{cComponents}}
%     \For{\text{segment in segmentAdjMatrix}}
%         \State \text{segmentsToConnect} $\gets$ \text{segmentAdjMatrix[segment]}
%         \For{\text{otherSegment in segmentsToConnect}}
%             % \State \text{connection} $\gets$ \Call{\text{extrapolate}}{\text{segment, otherSegment}}
%             \State \text{segment} $\gets$ \Call{\text{concat}}{\text{segment, otherSegment}} 
%             % \Comment{in-place merge}
%         \EndFor
%     \EndFor
%     \State \text{mergedSegments} $\gets$ \Call{\text{getNodes}}{\text{segmentAdjMatrix}} \Comment{mergedSegments contains our result}
% \end{algorithmic}
% \vspace{-2pt}
% \end{algorithm}
